# Supplementary material for: Latent Representation Prediction Networks
Source: arXiv:2009.09439 source file (2021-03-17)
Supplement: Supplementary file 1 [file Architecture_Appendix.pdf]

# S2 Appendix: TLDR Architectures

## Input

The networks $\phi$ encode the full NORB input to lower dimensional representations. The NORB input is $(96, 96, 1)$ so the input to the network at each time step is $(96, 96, 2)$ – the current viewpoint as well as the goal viewpoint. The inputs are not normalized beyond a scaling from [0, 255] integers to [0, 1] floats.

## Representation Learner $\phi$ Architecture

We use the same architecture for $\phi$ networks in all of our experiments except for varying the output dimension, Table 1.

**Table 1. TLDR network architecture.**

| Layer | Filters / Units | Kernel Size | Strides | Activation |
|---|---|---|---|---|
| Convolutional | 64 | $5 \times 5$ | $2 \times 2$ | ReLU |
| Max Pooling | | | $2 \times 2$ | |
| Convolutional | 128 | $5 \times 5$ | $2 \times 2$ | ReLU |
| Flatten | | | | |
| Dense | 600 | | | ReLU |
| Dense | #Features | | | Linear |

## Regularizing Decoder Architecture $D$

The decoder network $D$ has the architecture listed in Table 2. It's designed to approximately inverse each operation in the original $\phi$ network.

**Table 2. TLDR decoder architecture.**

| Layer | Filters / Units | Kernel Size | Strides | Activation |
|---|---|---|---|---|
| Dense | 512 | | | ReLU |
| Batch Normalization | | | | |
| Dense | 12800 | | | ReLU |
| Batch Normalization | | | | |
| Reshape to (10, 10, 128) | | | | |
| Conv. Transpose | 128 | $5 \times 5$ | $2 \times 2$ | ReLU |
| Upsampling with Linear Interpolation | | | $2 \times 2$ | |
| Batch Normalization | | | | |
| Conv. Transpose | 64 | $5 \times 5$ | $2 \times 2$ | ReLU |
| Batch Normalization | | | | |
| Conv. Transpose | 1 | $2 \times 2$ | $1 \times 1$ | Sigmoid |

## Predictor Network $f$

The predictor network $f$ is a two-stream dense neural network. Each stream consists of a dense layer followed by a batch normalization (BatchNorm) layer. The outputs of these streams are then concatenated and passed through 3 dense layers, each one followed by a BatchNorm, and then an output dense layer. Every dense layer, except the last, is followed by a rectified linear unit (ReLU) activation. Due to the non-sequential processing in the network, we depict it in Fig 1) instead of a table.

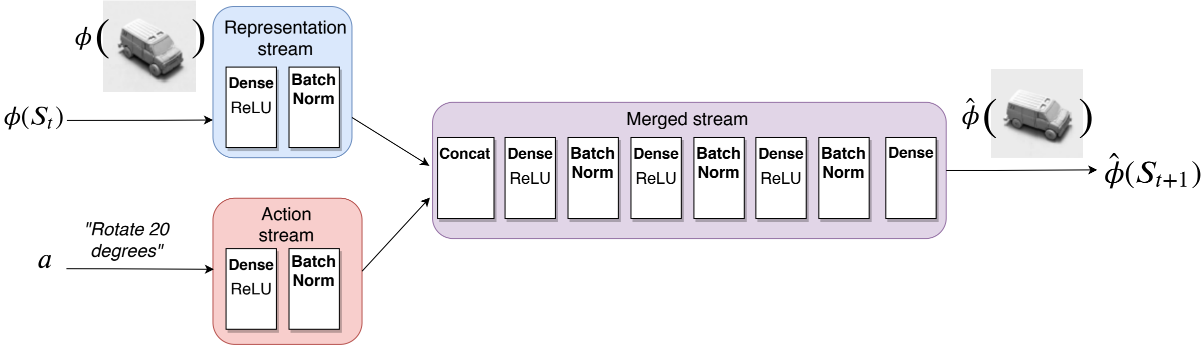


**Fig 1. Predictor net architecture.** The network takes as input the representation vector $\phi(S_t)$ of the state $S_t$ as determined by the feature map $\phi$, as well as the one-hot encoded action $a$. It outputs the estimated feature vector of the resulting state $S_{t+1}$ after action $a$ is performed. All dense layers have 256 hidden units except for the action stream dense layer and the final merged stream one, which have 128 units
