# Supplementary material for: Latent Representation Prediction Networks
Source: arXiv:2009.09439 source file (2021-03-17)
Supplement: Supplementary file 2 [file s2_network_keras_code.pdf]

# S2 Appendix: LARP Network Code

## Representation Learner $\phi$ Code

Below is Keras code for the $\phi$ module

```
def phi_net(coding_length, mode):
    inp = Input(shape=(96*96,))
    l1 = Reshape(target_shape=(int(np.sqrt(96*96)),
        int(np.sqrt(96*96)), 1))
    l2 = Conv2D(filters=int(64), kernel_size=5,
        strides=(2, 2), activation='relu')
    l3 = MaxPooling2D()
    l4 = Conv2D(filters=int(128), kernel_size=5,
        strides=(2, 2), activation='relu')
    l5 = Flatten()
    l6 = Dense(600, activation='relu')
    l7 = Dense(coding_length, name="phi")
    phi_out = l7(l6(l5(l4(l3(l2(l1(inp)))))))
    if mode == "l2_norm":
        norm = Lambda(lambda x: K.l2_normalize(x,axis=-1),
            name="l2_norm")
        phi_out = norm(phi_out)
    elif mode == "sphering":
        sphering = Sphering(output_dim=coding_length)
        phi_out = sphering(phi_out)
    return phi_out
```

## Regularizing Decoder Architecture $D$

A Keras code snipppet for the decoder is below

```
    decoder = Sequential([
    Dense(512, input_dim=coding_length, activation='relu'),
    Dense(10*10*128, activation="relu"),
    BatchNormalization(),
    Reshape(target_shape=(10, 10, 128)),
    BatchNormalization(),
    Conv2DTranspose(filters=128, kernel_size=5, strides=(2,
        2), padding="VALID", activation='relu'),
    UpSampling2D(),
    BatchNormalization(),
    Conv2DTranspose(filters=int(64*alpha), kernel_size=5,
    strides=(2, 2), padding="VALID", activation='relu'),
    BatchNormalization(),
    Conv2DTranspose(filters=1, kernel_size=2,  strides=(1,
        1), padding="VALID", activation="sigmoid"),
    Flatten(name="decoder")
])
```

## Predictor Network $f$

Keras code for the predictor:

```
inp_dense = Dense(int(256*alpha_f),
    activation=activation, name="f1")(phi_out_positive)
inp_dense =  BatchNormalization(name="f2")(inp_dense)
action_input =  Input(shape=(len(allowed_actions),),
    name='f3')
action_dense0 = Dense(int(128*alpha_f),
    activation=activation, name="f4")(action_input)
action_out = BatchNormalization(name="f5")(action_dense0)
conc = keras.layers.concatenate([action_out, inp_dense])
conc_dense0 = Dense(int(256*alpha_f),
    name='f6', activation="relu")(conc)
conc_dense0 = BatchNormalization(name='f7')(conc_dense0)
conc_dense1 = Dense(int(256*alpha_f),
    activation=activation, name="f8")(conc_dense0)
conc_dense1 = BatchNormalization(name="f9")(conc_dense1)
conc_dense2 = Dense(int(128*alpha_f),
    activation=activation, name="f10")(conc_dense1)
conc_dense2 =   BatchNormalization(name="f11")(conc_dense2)
out_dense = Dense(coding_length,
    activation="linear", name="f12")(conc_dense2)
out_dense = norm4(out_dense)
if mode == "decoder":
    out_conc = Concatenate()([out_dense,
        phi_out_anchor, phi_out_negative,
        decoder(phi_out_anchor), after_inp])
    f = Model([pos_inp, action_input,
        after_inp, neg_inp], out_conc)
else:
    out_conc = Concatenate()([out_dense,
        phi_out_anchor, phi_out_negative])
    f = Model([pos_inp, action_input, after_inp,
        neg_inp], out_conc)
f.compile(optimizer=keras.optimizers.RMSprop(lr=5E-5,
    rho=0.9), loss=custom_loss)
```

## Loss Function

Since loss functions in Keras always assume a "ground truth" input, even for unsupervised learning problems, we need to pass an unused dummy input to the loss function:

```
def custom_loss(yTrue, yPred):
    predicted_state_after = yPred[:, :coding_length]
    actual_state_after    = yPred[:,
        coding_length:2*coding_length]
    negative_state        = yPred[:,
        2*coding_length:3*coding_length]
    margin = .2
    positive = predicted_state_after
    anchor = actual_state_after
```

```
negative = negative_state
pos_dist = K.sum(K.square(anchor-positive),axis=-1)
neg_dist = K.sum(K.square(anchor-negative),axis=-1)
if mode == "decoder":
    recons_original_s  = yPred[:,
       3*coding_length:(3*coding_length+96*96)]
    actual_original_state = yPred[:,
       (3*coding_length+9216):(3*coding_length+9216*2)]
    loss = MSE(positive, anchor) + \
       K.sum(K.binary_crossentropy(recons_original_s,
       actual_original_state), axis=-1)
else:
    loss = pos_dist+K.maximum(-neg_dist+margin, 0)
return loss
```
